# Supplementary material for: SWE-VERIFIER: Selective Verification for Cost-Efficient Coding Agents
Source: arXiv:2610.30284 source file (2026-10-21)
Supplement: Supplementary file 1 [file appendix_style_grouped.tex]

\makeatletter
\@ifpackageloaded{xcolor}{}{\RequirePackage[table]{xcolor}}
\@ifpackageloaded{colortbl}{}{\RequirePackage{colortbl}}
\@ifpackageloaded{tcolorbox}{}{\RequirePackage[most]{tcolorbox}}
\@ifpackageloaded{tabularx}{}{\RequirePackage{tabularx}}
\@ifpackageloaded{array}{}{\RequirePackage{array}}
\@ifpackageloaded{enumitem}{}{\RequirePackage{enumitem}}
\@ifpackageloaded{fvextra}{}{\RequirePackage{fvextra}}
\@ifpackageloaded{caption}{}{\RequirePackage{caption}}
\@ifpackageloaded{booktabs}{}{\RequirePackage{booktabs}}
\@ifpackageloaded{stfloats}{}{\RequirePackage{stfloats}}
\@ifpackageloaded{placeins}{}{\RequirePackage{placeins}}
\providecommand\@setmarks{}
\makeatother

\tcbuselibrary{skins,breakable,raster}

\renewcommand{\arraystretch}{1.10}
\setlength{\tabcolsep}{3.5pt}
\setlength{\textfloatsep}{4pt plus 1pt minus 1pt}
\setlength{\dbltextfloatsep}{4pt plus 1pt minus 1pt}
\setlength{\floatsep}{4pt plus 1pt minus 1pt}
\setlength{\intextsep}{4pt plus 1pt minus 1pt}
\captionsetup{font=small,skip=0pt,hypcap=false}
\raggedbottom

\setcounter{topnumber}{5}
\setcounter{dbltopnumber}{5}
\setcounter{bottomnumber}{5}
\setcounter{totalnumber}{8}
\renewcommand{\topfraction}{0.98}
\renewcommand{\bottomfraction}{0.98}
\renewcommand{\dbltopfraction}{0.98}
\renewcommand{\textfraction}{0.02}
\renewcommand{\floatpagefraction}{0.88}
\renewcommand{\dblfloatpagefraction}{0.88}

\makeatletter
\setlength{\@fptop}{0pt}
\setlength{\@fpsep}{6pt plus 1fil}
\setlength{\@fpbot}{0pt plus 1fil}
\setlength{\@dblfptop}{0pt}
\setlength{\@dblfpsep}{6pt plus 1fil}
\setlength{\@dblfpbot}{0pt plus 1fil}
\makeatother

\definecolor{HeaderGray}{HTML}{1F2328}
\definecolor{OuterBack}{HTML}{FCFCFD}
\definecolor{RuleGray}{HTML}{B7BEC8}
\definecolor{TableHeader}{HTML}{DDEBFA}
\definecolor{TableStripe}{HTML}{F7F9FC}

\definecolor{SystemFrame}{HTML}{6E40C9}
\definecolor{PromptFrame}{HTML}{8A5A18}
\definecolor{ActionFrame}{HTML}{0969DA}
\definecolor{ObsFrame}{HTML}{1A7F37}
\definecolor{CandFrame}{HTML}{4D5562}
\definecolor{TeacherFrame}{HTML}{B42318}
\definecolor{PatchFrame}{HTML}{CF222E}
\definecolor{DecisionFrame}{HTML}{0A7B83}
\definecolor{TakeFrame}{HTML}{6639BA}
\definecolor{CorrectFrame}{HTML}{1A7F37}
\definecolor{IncorrectFrame}{HTML}{CF222E}

\definecolor{SystemBack}{HTML}{F6F0FF}
\definecolor{PromptBack}{HTML}{FFF7EA}
\definecolor{ActionBack}{HTML}{EEF6FF}
\definecolor{ObsBack}{HTML}{F0FAF2}
\definecolor{CandBack}{HTML}{F3F5F8}
\definecolor{TeacherBack}{HTML}{FFF4F2}
\definecolor{PatchBack}{HTML}{FFF1F1}
\definecolor{DecisionBack}{HTML}{EAFBFA}
\definecolor{TakeBack}{HTML}{F4F0FF}
\definecolor{CorrectBack}{HTML}{E8FFEE}
\definecolor{IncorrectBack}{HTML}{FFEBE9}

\colorlet{LightGray}{OuterBack}
\colorlet{BoxBack}{OuterBack}

\newenvironment{trajwidefig}[3]%
{%
  \def\trajcaptiontext{#2}%
  \def\trajlabelname{#3}%
  \begin{figure*}[!tbp]
  \centering
  \begin{minipage}{0.995\textwidth}
  \begin{tcolorbox}[
    enhanced,
    colback=OuterBack,
    colframe=HeaderGray,
    coltitle=white,
    colbacktitle=HeaderGray,
    title={#1},
    fonttitle=\bfseries\small,
    boxrule=0.75pt,
    arc=0.7mm,
    left=0.75mm,
    right=0.75mm,
    top=0.35mm,
    bottom=0.35mm,
    before skip=0pt,
    after skip=0pt,
    borderline west={1.8pt}{0pt}{HeaderGray}
  ]
}%
{%
  \end{tcolorbox}
  \caption{\trajcaptiontext}
  \label{\trajlabelname}
  \end{minipage}
  \end{figure*}
}

\newenvironment{trajwidefigcontinued}[2]%
{%
  \def\trajcontcaptiontext{#2}%
  \begin{figure*}[!tbp]
  \ContinuedFloat
  \centering
  \begin{minipage}{0.995\textwidth}
  \begin{tcolorbox}[
    enhanced,
    colback=OuterBack,
    colframe=HeaderGray,
    coltitle=white,
    colbacktitle=HeaderGray,
    title={#1},
    fonttitle=\bfseries\small,
    boxrule=0.75pt,
    arc=0.7mm,
    left=0.75mm,
    right=0.75mm,
    top=0.35mm,
    bottom=0.35mm,
    before skip=0pt,
    after skip=0pt,
    borderline west={1.8pt}{0pt}{HeaderGray}
  ]
}%
{%
  \end{tcolorbox}
  \vspace{-0.35em}
  \end{minipage}
  \end{figure*}
}

\newenvironment{widefigure}[2]%
{%
  \def\widefigcaption{#1}%
  \def\widefiglabel{#2}%
  \begin{figure*}[!tbp]
  \centering
  \begin{minipage}{0.995\textwidth}
  \centering
}%
{%
  \caption{\widefigcaption}
  \label{\widefiglabel}
  \end{minipage}
  \end{figure*}
}

\newenvironment{widecenter}
{%
  \begin{figure*}[!tbp]
  \centering
  \begin{minipage}{0.995\textwidth}
  \centering
}
{%
  \end{minipage}
  \end{figure*}
}

\newtcolorbox{trajgroup}[2][]{
  enhanced,
  colback=OuterBack,
  colframe=HeaderGray,
  coltitle=white,
  colbacktitle=HeaderGray,
  title={#2},
  fonttitle=\bfseries\small,
  boxrule=0.70pt,
  arc=0.7mm,
  left=0.9mm,
  right=0.9mm,
  top=0.7mm,
  bottom=0.7mm,
  before skip=0.35em,
  after skip=0.35em,
  borderline west={1.4pt}{0pt}{HeaderGray},
  #1
}

\newtcolorbox{compactsummary}[2][]{
  enhanced,
  colback=OuterBack,
  colframe=RuleGray,
  coltitle=white,
  colbacktitle=HeaderGray,
  title={#2},
  fonttitle=\bfseries\scriptsize,
  boxrule=0.45pt,
  arc=0.6mm,
  left=0.9mm,
  right=0.9mm,
  top=0.55mm,
  bottom=0.55mm,
  before skip=0.35em,
  after skip=0.35em,
  #1
}

\newcommand{\legenditem}[4]{%
  \noindent\tcbox[on line,enhanced,boxrule=0pt,arc=0.5mm,left=0.8mm,right=0.8mm,top=0.25mm,bottom=0.25mm,colback=#1,colframe=#1,coltext=white]{\scriptsize\bfseries #2}%
  \hspace{0.35em}{\footnotesize #3}\par\vspace{0.15em}%
}

\newenvironment{trajwide}[2][]
  {\begin{trajwidefig}{#2}{#2}{fig:unlabeled-trajwide}}
  {\end{trajwidefig}}
\newenvironment{widetrajgroup}[2][]
  {\begin{trajwidefig}{#2}{#2}{fig:unlabeled-widetraj}}
  {\end{trajwidefig}}
\newenvironment{trajectorygroup}[2][]
  {\begin{trajgroup}[#1]{#2}}
  {\end{trajgroup}}

\newenvironment{trajseg}[3]
{%
  \begin{tcolorbox}[
    enhanced,
      colback=#2,
    colframe=#3,
    coltitle=white,
    colbacktitle=#3,
    title={#1},
    fonttitle=\bfseries\scriptsize,
    boxrule=0.30pt,
    arc=0.55mm,
    left=0.85mm,
    right=0.85mm,
    top=0.25mm,
    bottom=0.25mm,
    before skip=0.055em,
    after skip=0.055em,
    titlerule=0pt,
    toptitle=0.18mm,
    bottomtitle=0.18mm,
    borderline west={1.05pt}{0pt}{#3}
  ]
}
{%
  \end{tcolorbox}
}

\newenvironment{trajgrid}
{\begin{tcbraster}[raster columns=2,raster equal height=none,raster column skip=1.0mm,raster row skip=0.35mm,raster valign=top]}
{\end{tcbraster}}

\newenvironment{candidategrid}
{\begin{tcbraster}[raster columns=2,raster equal height=none,raster column skip=1.0mm,raster row skip=0.40mm,raster valign=top]}
{\end{tcbraster}}

\newtcolorbox{candidatecard}[2][]{
  enhanced,
  colback=CandBack,
  colframe=CandFrame,
  coltitle=white,
  colbacktitle=CandFrame,
  title={#2},
  fonttitle=\bfseries\scriptsize,
  boxrule=0.35pt,
  arc=0.55mm,
  left=0.85mm,
  right=0.85mm,
  top=0.30mm,
  bottom=0.30mm,
  before skip=0pt,
  after skip=0pt,
  titlerule=0pt,
  toptitle=0.25mm,
  bottomtitle=0.25mm,
  borderline west={1.05pt}{0pt}{CandFrame},
  #1
}

\newcommand{\teacherchoice}[1]{%
  \begin{tcolorbox}[
    enhanced,
    colback=TeacherBack,
    colframe=TeacherFrame,
    boxrule=0.45pt,
    arc=0.6mm,
    left=0.9mm,right=0.9mm,top=0.4mm,bottom=0.4mm,
    before skip=0.10em,after skip=0.25em,
    borderline west={1.4pt}{0pt}{TeacherFrame}
  ]
  {\footnotesize\bfseries #1}
  \end{tcolorbox}%
}

\newenvironment{teachercomparison}
{\begin{tcbraster}[raster columns=2,raster equal height=none,raster column skip=1.1mm,raster row skip=0.35mm,raster valign=top]}
{\end{tcbraster}}

\newtcolorbox{verifierbox}[3][]{
  enhanced,
  colback=TeacherBack,
  colframe=#3,
  coltitle=white,
  colbacktitle=#3,
  title={#2},
  fonttitle=\bfseries\scriptsize,
  boxrule=0.45pt,
  arc=0.65mm,
  left=0.8mm,
  right=0.8mm,
  top=0.32mm,
  bottom=0.32mm,
  before skip=0pt,
  after skip=0pt,
  titlerule=0pt,
  toptitle=0.28mm,
  bottomtitle=0.28mm,
  borderline west={1.15pt}{0pt}{#3},
  #1
}

\newtcolorbox{teachercard}[3][]{
  enhanced,
  colback=white,
  colframe=RuleGray,
  coltitle=HeaderGray,
  colbacktitle=TeacherBack,
  title={#2 \hfill \normalfont #3},
  fonttitle=\bfseries\scriptsize,
  fontupper=\fontsize{7.45pt}{7.85pt}\selectfont,
  boxrule=0.28pt,
  arc=0.50mm,
  left=0.75mm,
  right=0.75mm,
  top=0.25mm,
  bottom=0.25mm,
  before skip=0.09em,
  after skip=0.09em,
  titlerule=0pt,
  toptitle=0.22mm,
  bottomtitle=0.22mm,
  #1
}

\newtcolorbox{teachercardwide}[3][]{
  enhanced,
  colback=white,
  colframe=RuleGray,
  coltitle=HeaderGray,
  colbacktitle=TeacherBack,
  title={#2 \hfill \normalfont #3},
  fonttitle=\bfseries\scriptsize,
  fontupper=\fontsize{7.45pt}{7.85pt}\selectfont,
  boxrule=0.28pt,
  arc=0.50mm,
  left=0.75mm,
  right=0.75mm,
  top=0.25mm,
  bottom=0.25mm,
  before skip=0.14em,
  after skip=0.14em,
  titlerule=0pt,
  toptitle=0.22mm,
  bottomtitle=0.22mm,
  #1
}


\newcommand{\fivechecks}[5]{%
  \par\vspace{0.06em}\noindent{\fontsize{6.6pt}{7.0pt}\selectfont
  \textbf{Checklist scores:}\enspace C1=#1,\enspace C2=#2,\enspace C3=#3,\enspace C4=#4,\enspace C5=#5}%
  \par\vspace{0.05em}%
}

\newcommand{\field}[1]{\par\vspace{0.07em}\noindent{\scriptsize\bfseries\textcolor{HeaderGray}{#1.}}\hspace{0.25em}}

\newtcolorbox{decisiontext}[2][]{
  enhanced,
  colback=DecisionBack,
  colframe=DecisionFrame,
  coltitle=white,
  colbacktitle=DecisionFrame,
  title={#2},
  fonttitle=\bfseries\scriptsize,
  boxrule=0.55pt,
  arc=0.7mm,
  left=0.9mm,
  right=0.9mm,
  top=0.50mm,
  bottom=0.50mm,
  before skip=0pt,
  after skip=0pt,
  borderline west={1.4pt}{0pt}{DecisionFrame},
  #1
}

\newtcolorbox{takeawaybox}[2][]{
  enhanced,
  colback=TakeBack,
  colframe=TakeFrame,
  coltitle=white,
  colbacktitle=TakeFrame,
  title={#2},
  fonttitle=\bfseries\scriptsize,
  boxrule=0.55pt,
  arc=0.7mm,
  left=0.9mm,
  right=0.9mm,
  top=0.55mm,
  bottom=0.55mm,
  before skip=0.35em,
  after skip=0.35em,
  borderline west={1.4pt}{0pt}{TakeFrame},
  #1
}

\newenvironment{TrajVerbatim}
{\VerbatimEnvironment
 \begin{Verbatim}[
   fontsize=\fontsize{6.65pt}{7.05pt}\selectfont,
   breaklines=true,
   breakanywhere=true,
   breakindent=0pt,
   breakautoindent=false,
   breaksymbolleft={},
   breaksymbolright={},
   xleftmargin=0pt,
   xrightmargin=0pt,
   tabsize=2
 ]}
{\end{Verbatim}}
\newenvironment{trajverbatim}{\begin{TrajVerbatim}}{\end{TrajVerbatim}}

\newenvironment{DenseText}
{\fontsize{7.45pt}{7.85pt}\selectfont\setlength{\parindent}{0pt}\setlength{\parskip}{0.025em}}
{}

\newcommand{\good}[1]{\textcolor{CorrectFrame}{\textbf{#1}}}
\newcommand{\bad}[1]{\textcolor{IncorrectFrame}{\textbf{#1}}}
\newcommand{\neutral}[1]{\textcolor{HeaderGray}{\textbf{#1}}}
\newcommand{\correctrow}{\rowcolor{CorrectBack}}
\newcommand{\incorrectrow}{\rowcolor{IncorrectBack}}



\usepackage{fvextra}
\tcbuselibrary{breakable,skins}

\DefineVerbatimEnvironment{PromptVerbatim}{Verbatim}{
  fontsize=\scriptsize,
  breaklines=true,
  breakanywhere=true,
  breaksymbolleft={},
  breaksymbolright={},
  tabsize=2
}

\newtcolorbox{promptbox}[1]{
  enhanced,
  breakable,
  colback=gray!3,
  colframe=black!70,
  colbacktitle=black!80,
  coltitle=white,
  title={#1},
  fonttitle=\bfseries\small,
  boxrule=0.6pt,
  arc=0.8mm,
  left=1mm,
  right=1mm,
  top=0.6mm,
  bottom=0.6mm,
  before skip=0.6em,
  after skip=0.8em
}
